# Supplementary material for: Striped Magnetic Ground State of the Kagome Lattice in Fe4Si2Sn7O16
Source: arXiv:1703.08637 ancillary file (2017-10-27)
Supplement: Supplementary file 1 [file SM.pdf]

# Supplementary Information

A sample of $Fe_4Si_2Sn_7O_{16}$ was prepared as reported previously. [1, 2] Temperature-dependent DC magnetic susceptibility measurements were carried out under field-cooled and zero-field-cooled conditions using the vibrating sample magnetometer (VSM) attachment of a Quantum Design Physical Properties Measurement System (PPMS), in an applied field of 0.1 T, between room temperature and 1.9 K. Field-dependent magnetization data to $B = \pm 9$ T were also collected above and below $T_N$ on the same instrument. Data are shown in Fig. 1. A downturn in the temperature-dependent susceptibility is clearly seen at $T_N = 3.5$ K, highlighted in the inset to Fig. 1. There is no significant divergence between the zero-field-cooled and field-cooled curves, i.e., no evidence for spin-glass behavior; and no significant inflection or opening of field-dependent susceptibility curves above or below $T_N$, i.e., no sign of a field-induced transition or of a ferromagnetic (FM) component to the ground state (Fig. 2). A Curie-Weiss fit to the inverse susceptibility in the paramagnetic regime (above 30 K) yields an effective magnetic moment $\mu_{\text{eff}} = 5.45\ \mu_B$ per HS $Fe^{2+}$ (Fig. 3). This is slightly higher than the spin-only moment $\mu_{\text{so}} = 4.90\ \mu_B$, but in the normal range for HS $Fe^{2+}$ which always shows incomplete quenching of the orbital contribution. The Weiss temperature $\theta = -12.7$ K corresponds to a modest frustration index [3] $f = |\theta/T_N| = 3.6$.

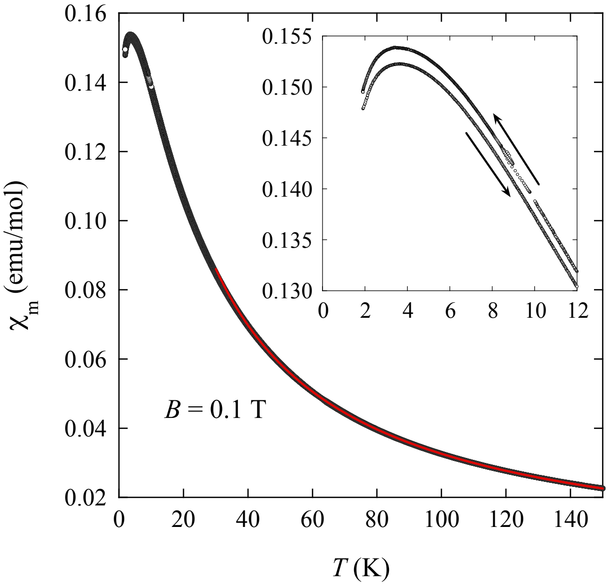


FIG. 1. Field-cooled/zero-field-cooled magnetic susceptibility in a 0.1 T field for $Fe_4Si_2Sn_7O_{16}$. The red line is a Curie-Weiss fit to the zero-field-cooled data. The inset highlights the downturn at $T_N = 3.5$ K.

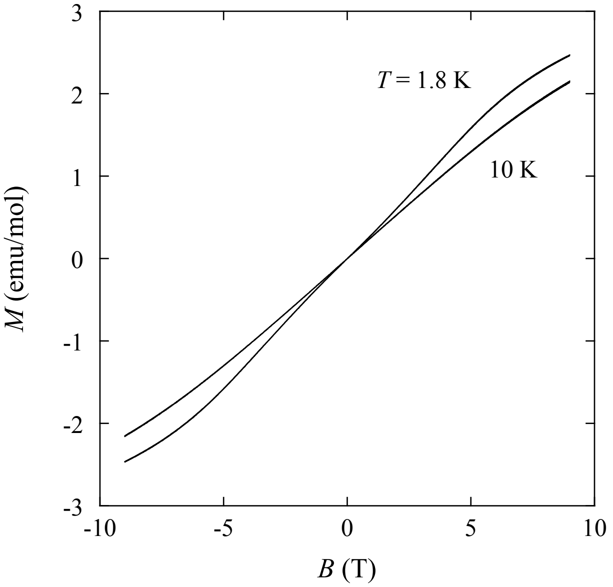


FIG. 2. Field-dependent magnetization above and below $T_N$ for $Fe_4Si_2Sn_7O_{16}$.

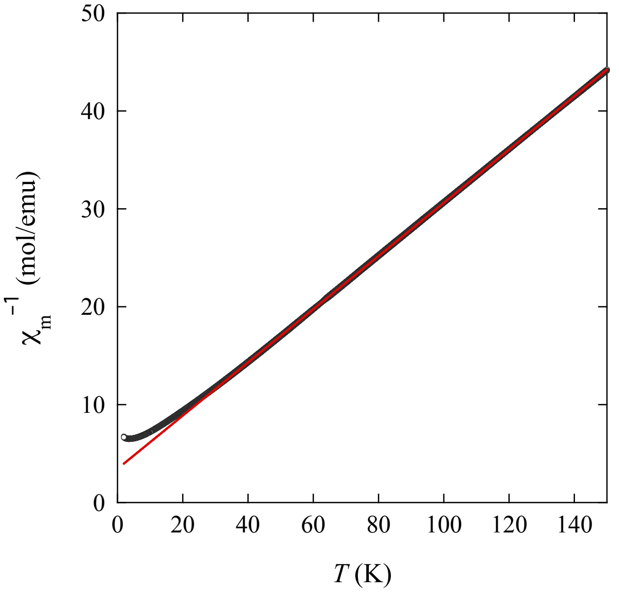


FIG. 3. Field-cooled/zero-field-cooled inverse magnetic susceptibility in a 0.1 T field for $Fe_4Si_2Sn_7O_{16}$. The red line is a Curie-Weiss fit to the zero-field-cooled data above 30 K.

Fig. 4(a) shows the emergence of new low-angle Bragg peaks for $Fe_4Si_2Sn_7O_{16}$ at 1.6 K, below $T_N$, indicative of 3D long-range-ordered magnetism. Fig. 4(b) shows the same peaks at 0.1 K, i.e., the magnetic structure shows no further change down to at least this temperature. Additional features in the latter data come from Al and Cu metal in the dilution insert and cryostat heat shield respectively. Fig. 4(c) shows the same peaks again at 1.8

K for $Fe_{1.45}Mn_{2.55}Si_2Sn_7O_{16}$.

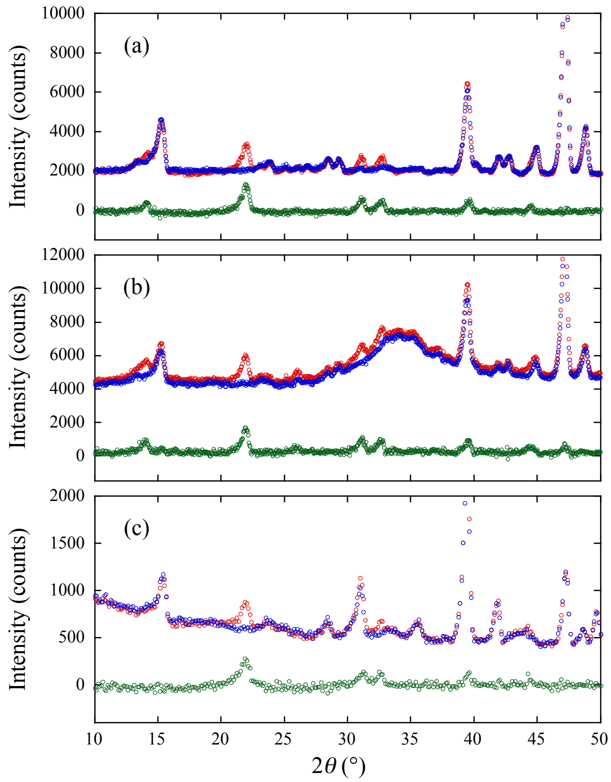


FIG. 4. NPD data above (blue) and below (red) $T_N$ and the difference between them (green). (a) $Fe_4Si_2Sn_7O_{16}$ at 1.6 and 10 K and (b) 0.1 and 3.5 K (additional background is the dilution insert). (c) $Fe_{1.45}Mn_{2.55}Si_2Sn_7O_{16}$ at 1.8 and 5.0 K.

The basis vectors for the magnetic structure of $Fe_4Si_2Sn_7O_{16}$ are given in Table I.

TABLE I. Representation analysis for the magnetic Fe atom on the 3f Wyckoff site of space group $P\bar{3}m1$ and a propagation vector $q = (0, \frac{1}{2}, \frac{1}{2})$.

| Irrep | Fe-3f(1) | $\text{Fe-3f(2)}_1$ | $\text{Fe-3f(2)}_2$ |
|---|---|---|---|
| | $x+\frac{1}{2}, y+\frac{1}{2}, z$ | $x, y, z$ | $x-y, -y, -z$ |
| | | (1 0 0) | (1 0 0) |
| $\Gamma_1$ | | (0 1 0) | $(\bar{1}\ \bar{1}\ 0)$ |
| | | (0 0 1) | $(0\ 0\ \bar{1})$ |
| $\Gamma_2$ | (1 2 0) | | |
| | (0 0 1) | | |
| | | (1 0 0) | $(\bar{1}\ 0\ 0)$ |
| $\Gamma_3$ | | (0 1 0) | (1 1 0) |
| | | (0 0 1) | (0 0 1) |
| $\Gamma_4$ | (1 0 0) | | |

[1] T. Söhnel, P. Böttcher, W. Reichelt, and F. Wagner, Z. Anorg. Allg. Chem. **624**, 708 (1998).
[2] M. C. Allison, M. Avdeev, S. Schmid, S. Liu, T. Söhnel, and C. D. Ling, Dalton Trans. **45**, 9689 (2016).
[3] A. P. Ramirez, Annu. Rev. Mater. Sci. **24**, 453 (1996).
